# Supplementary material for: Neighbourhood watch in mechanics: non-local models and convolution
Source: arXiv:2306.15674 source file (2023-05-20)
Supplement: Supplementary file 1 [file references_supplement.tex]

\begin{thebibliography}{1}

\bibitem{bronstein2012taschenbuch}
{\sc I.~N. Bronstein, J.~Hromkovic, B.~Luderer, H.-R. Schwarz, J.~Blath,
  A.~Schied, S.~Dempe, G.~Wanka, and S.~Gottwald}, {\em Taschenbuch der
  Mathematik}, vol.~1, Springer-Verlag, 2012.

\bibitem{dorf2017modern}
{\sc R.~Dorf and R.~Bishop}, {\em Modern Control Systems}, Pearson, 2017.

\bibitem{haupt2013continuum}
{\sc P.~Haupt}, {\em Continuum mechanics and theory of materials}, Springer
  Science \& Business Media, 2013.

\bibitem{krawietz2013materialtheorie}
{\sc A.~Krawietz}, {\em Materialtheorie: mathematische Beschreibung des
  ph{\"a}nomenologischen thermomechanischen Verhaltens}, Springer-Verlag, 2013.

\bibitem{oppenheim2013discrete}
{\sc A.~Oppenheim, R.~Schafer, and J.~Buck}, {\em Discrete-time Signal
  Processing}, Prentice-Hall signal processing series, Pearson, 2013.

\bibitem{robinson1957predictive}
{\sc E.~A. Robinson}, {\em Predictive decomposition of seismic traces},
  Geophysics, 22 (1957), pp.~767--778,
  \url{https://doi.org/https://doi.org/10.1190/1.1438415}.

\bibitem{stengel2012optimal}
{\sc R.~Stengel}, {\em Optimal Control and Estimation}, Dover Books on
  Mathematics, Dover Publications, 2012.

\end{thebibliography}
